# Supplementary material for: Functional Limit Theorems for Marked Hawkes Point Measures
Source: arXiv:1908.06703 source file (2019-08-19)
Supplement: Supplementary file 1 [file Appendix.tex]

\bigskip
 \appendix
 \centerline{\textsc{\Large  Appendix: Weak Convergence of Error Processes}}

 \section{Proof for Lemma~\ref{Thm502.03}}\label{AppendixA}
 \setcounter{equation}{0}
 
 In this section, we mainly prove the weak convergence of error processes $\{ \varepsilon^\kappa_{T,H} (\cdot)\}_{T\geq 0}$ to $0$ with $\kappa=1$ under Condition~\ref{C1}.
 The proof for the sequence $\{ \varepsilon^\kappa_{T,I}(\cdot) \}_{T\geq 0}$ is similar and much simpler.
 For any $T>0$, let $\delta_T=T^{-\beta}$ for some $\beta\in(\frac{1}{\alpha}, 1-\frac{1}{2\theta_0})$.
 We split the error process  $\varepsilon^1_{T,H}(\cdot)$ into the following two parts:
 \beqlb
 \varepsilon_{T,H,1}(t)
 \ar:=\ar \frac{1}{\sqrt{T}}  \int_0^{t-\delta_T} \int_{\mathbb{U}}  \int_0^{Z(Ts-)}
 \int_{T(t-s)}^\infty R(r,u)dr\tilde{N}_0(dTs,du,dz),  \label{eqnA.01} \\
 \varepsilon_{T,H,2}(t)
 \ar:=\ar \frac{1}{\sqrt{T}} \int_{t-\delta_T}^t \int_{\mathbb{U}}   \int_0^{Z(Ts-)}
 \int_{T(t-s)}^\infty R(r,u)dr\tilde{N}_0(dTs,du,dz)).\label{eqnA.02}
 \eeqlb
 We first prove  the sequence $\{\varepsilon_{T,0,1}(\cdot)\}_{T\geq 0}$ converges to $0$ uniformly in probability on any bounded interval.
 
 \begin{corollary}\label{ThmA01}
 	There exists a constant $C>0$ such that for any $t\geq 0$ and $i=0,1$,
 	\beqlb\label{eqnA.03}
 	\int_t^{\infty} R_i(s)ds  \leq  Ct^{-\theta}.
 	\eeqlb
 \end{corollary}
 \proof
 %From Assumption~\ref{C1}(2), we can always find a nonnegative, non-increasing function $f(t)$ satisfying that
 %\beqnn
 % f(t)\in \mathrm{RV}_{-\theta}, \quad \phi_\Lambda(t)\leq f(t) \quad \mbox{and}\quad   \|f\|_{L_1}:=\int_0^\infty f(t)dt<\frac{1}{m_0}.
 %%\eeqnn
 %From (\ref{eqn3.03}), we have
 %\beqnn
 %R_0(t)\ar \leq\ar m_0 f(t)+  m_0\int_0^t R_0(t-s) f(s) ds.
 %\eeqnn
 %By the Gr\"onwall's ineqaulity in Chu and Metcalf (1966),
 %\beqnn
 %R_0(t)\leq \sum_{i=1}^\infty (m_0 f)^{(i)}(t),\quad \mbox{for any } t\geq 0,
 % \eeqnn
 % where $(m_0 f)^{(i)}$ is the $i$-fold convolution of $m_0 f(\cdot)$.
 Let $\{X_k\}_{k\geq 1}$ be a sequence of i.i.d. random variables with probability density function $\hat{f}(t):= \phi_0(t)/\|\phi_0\|_{L_1}$ and $N_G$  be a geometric random variable with parameter $1-   \|\phi_0\|_{L_1}>0$ independent of $\{X_k\}_{k\geq 1}$.
 From the one-to-one correspondence  between probability law and its Laplace transform, it is easy to see the geometric summation $\sum_{k=1}^{N_G}X_k$ has the following probability density
 \beqlb
 \frac{1-\|\phi_0\|_{L_1}}{\|\phi_0\|_{L_1}} \sum_{i=1}^\infty  \phi_0^{(*i)}(t)
 = \frac{1-\|\phi_0\|_{L_1}}{\|\phi_0\|_{L_1}} R_0(t) . \label{eqnA.03.1}
 \eeqlb
 From Condition~\ref{C1}, this geometric summation has finite $\theta$-th moment, i.e. $\mathbf{E}[|\sum_{k=1}^{N_G}X_k|^\theta]<\infty$.
 From Markov's inequality, there exits a constant $C>0$ such that for  any $t>0$,
 \beqnn
 \mathbf{P}\Big\{ \sum_{k=1}^{N_G}X_k  >t\Big\}
 \leq \mathbf{E}\Big[\Big|\sum_{k=1}^{N_G}X_k\Big|^\theta\Big]t^{-\theta}
 \leq Ct^{-\theta}.
 \eeqnn
 Taking this estimate back into (\ref{eqnA.03.1}), we have
 \beqnn
 \int_t^\infty  R_0(s)ds \leq C\mathbf{P}\Big\{ \sum_{k=1}^{N_G}X_k  >t\Big\}\leq Ct^{-\theta}.
 \eeqnn
 Here we have gotten the desired result for $i=0$.
 For the case $i=1$, from (\ref{eqn2.10}) we have
 \beqnn
 R_1(t)\ar=\ar \phi_1(t)+\frac{\|\phi_0\|_{L^1}\|\phi_1\|_{L^1}} {1-\|\phi_0\|_{L^1}} \int_0^t \frac{1-\|\phi_0\|_{L^1}}{\|\phi_0\|_{L^1}} R_0(t-s) \times \frac{\phi_1(s)}{\|\phi_1\|_{L^1}}ds
 \eeqnn
 Let $Y$ be an $\mathbb{R}_+$-valued random variable with  probability density $\phi_1(t)/\|\phi_1\|_{L^1}$ and independent of  the geometric summation $\sum_{k=1}^{N_G}X_k$. Thus the convolution in the above equation is consistent to the probability density of $\sum_{k=1}^{N_G}X_k+ Y$ whoes $\theta$-th moment is finite. Like the previous argument, we also have
 \beqnn
 \int_t^\infty R_1(s)ds \leq  t^\theta\int_t^\infty |\frac{s}{t}|^\theta\phi_1(s)ds + C \mathbf{P}\Big\{ \sum_{k=1}^{N_G}X_k+ Y \geq t\Big\} \leq C t^{-\theta}.
 \eeqnn
 Here we have finished the proof.
 \qed

 \begin{corollary}\label{ThmA02}
 	We have $  \sup_{t\in[0,1]} |\varepsilon_{T,H,1}(t)|\to 0$ in probability as $T\to\infty$
 \end{corollary}
 \proof From (\ref{eqnA.01}), we have 
 \beqnn
 |\varepsilon_{T,H,1}(t)|
 \ar\leq \ar  \sqrt{T} \int_0^{t-\delta_T} Z(Ts)ds \int_{\mathbb{U}}
 \int_{T^{1-\beta}}^\infty R(r,u)dr \nu_0(du)  \cr
 \ar\ar  + \frac{1}{\sqrt{T}} \int_0^{t-\delta_T} \int_{\mathbb{U}}  \int_0^{Z(Ts-)}
 \int_{T^{1-\beta}}^\infty R(r,u)dr N_0(dTs,du,dz).
 % \ar\leq\ar  \sqrt{T}\int_0^{1}Z(Ts)ds
 %  \int_{T^{1-\beta}}^\infty R_0(r)dr  \cr
 % \ar\ar +  \frac{1}{\sqrt{T}} \int_0^{1} \int_{\mathbb{U}\times\Psi}  \int_0^{Z(Ts-)}
 % \int_{T^{1-\beta}}^\infty R_0(r,u)dr N_0(dTs,du,d\psi,dz).
 \eeqnn
 Taking expectation on the both sides of the above inequality, from Lemma~\ref{Thm201} we have
 \beqnn
 \mathbf{E}\Big[\sup_{t\in[0,1]}|\varepsilon_{T,H,1}(t)|\Big]
 \ar\leq\ar C\sqrt{T}\int_0^{1} \mathbf{E}[Z(Ts)]ds
 \int_{T^{1-\beta}}^\infty R_0(r)dr
 \leq C\sqrt{T}\int_{T^{1-\beta}}^\infty R_0(r)dr.
 \eeqnn
 From Corollary~\ref{ThmA01} and $\beta<1-\frac{1}{2\theta}$, we have as $T\to\infty$,
 \beqnn
 \mathbf{E}\Big[\sup_{t\in[0,1]}|\varepsilon_{T,H,1}(t)|\Big]\leq C T^{1/2- (1-\beta)\theta}\to 0.
 \eeqnn
 Here we have finished the proof.
 \qed
 
 Now we start to prove the sequence $\{ \varepsilon_{T,H,2}(\cdot) \}_{T\geq 0}$ converges to $0$ weakly. It suffices to prove that it is tight in the space $\mathbb{D}([0,\infty),\mathbb{R})$ and converges $0$ in the sense of finite-dimensional distributions.
 
 \begin{corollary}\label{ThmA03}
 	The sequence $\{ \varepsilon_{T,H,2}(\cdot) \}_{T\geq 0}$ converges to $0$  in the sense of finite-dimensional distributions, i.e.  we have as $T\to\infty$,
 	\beqnn
 	\mathbf{E}\big[ |\varepsilon_{T,H,2}(t)|^{2}\big]\to 0, \quad \mbox{for any }t\geq 0.
 	\eeqnn
 \end{corollary}
 \proof From the  Burkholder-Davis-Gundy inequality, Lemma~\ref{Thm201} and (\ref{eqn4.07}), we have 
 \beqnn
 \mathbf{E}[ |\varepsilon_{T,H,2}(t)|^{2}]\ar\leq\ar \frac{C}{T}\mathbf{E}\Big[  \Big|   \int_{t-\delta_T}^t  \int_{\mathbb{U}}  \int_0^{Z(Ts-)}
 \Big|\int_{0}^\infty R(r,u)dr\Big|^2 N_0(dTs,du,dz)  \Big]\cr
 \ar\leq\ar C  \int_{t-\delta_T}^t   \mathbf{E}[Z(Ts)]ds  \int_{\mathbb{U}}
 \Big|\int_{0}^\infty R(r,u)dr\Big|^2 \nu_0(du) \leq CT^{-\beta},
 \eeqnn
 which vanishes as $T\to \infty$.
 \qed
 
 For the tightness of the sequence $\{ \varepsilon_{T,H,2}(\cdot) \}_{T\geq 0}$ ,  from Theorem~8.8 in Ethier and Kurtz (1989, p.139),
 it suffices to  prove that there exist two constants $\gamma>1$ and $C>0$ such that for any $T,h>0$,
 \beqlb\label{eqnA.04}
 \sup_{t\in[0,1]}\mathbf{E}\Big[ |\triangle_h\varepsilon_{T,H,2}(t)|^\alpha\times |\triangle_h\varepsilon_{T,H,2}(t+h)|^\alpha \Big]\leq Ch^{\gamma},
 \eeqlb
 where $\triangle_h f(t):=f(t)-f(t-h)$.
 As a preparation, we first give an upper bound for the second moments of the sequence.
 \begin{corollary}\label{ThmA04}
 	Under Condition~\ref{C1}, we have $\sup_{t\geq 0}\mathbf{E}[|Z(t)|^{2\alpha}]<\infty.$
 \end{corollary}
 \proof From (\ref{eqn5.01.07}) and the Cauchy-Schwarz inequality, we can see that for any $\kappa\in [1,\alpha]$,
 \beqlb\label{eqnA.05.2}
 \mathbf{E}[|Z(t)|^{2\kappa}]
 \ar\leq\ar C\mathbf{E}[|\mu_0(t)|^{2\kappa}]+ C\mathbf{E}\Big[\Big|\int_0^t R_0(t-s)\mu_0(s)ds\Big|^{2\kappa} \Big]\cr
 \ar\ar +C\mathbf{E}\Big[\Big|\int_0^t  \int_{\mathbb{U}}  R(t-s,u)\tilde{N}_I(ds,du)\Big|^{2\kappa} \Big] \cr
 \ar\ar + C\mathbf{E}\Big[ \Big|\int_0^t \int_{\mathbb{U}} \int_0^{Z(s-)} R(t-s,u)\tilde N_0(ds,du,dz)\Big|^{2\kappa} \Big].
 \eeqlb
 The uniform boundedness of the first term on the right side of the above inequality follows directly from Condition~\ref{C1}. For the second term, by H\"older's inequality,
 \beqnn
 \mathbf{E}\Big[\Big|\int_0^t R_0(t-s)\mu_0(s)ds\Big|^{2\kappa} \Big]\ar\leq\ar \Big(\int_0^t R_0(s)ds  \Big)^{2\kappa-1}\int_0^t R_0(t-s)\mathbf{E}[|\mu_0(s)|^{2\kappa}]ds,
 \eeqnn
 which is uniformly bounded.
 Now we prove the last expectation  in (\ref{eqnA.05.2}) is uniformly bounded and the second-to-last term can proved in this same way.
 From the Burkholder-Davis-Gundy inequality,
 \beqnn
 \mathbf{E}\Big[ \Big|\int_0^t \int_{\mathbb{U}} \int_0^{Z(s-)} R(t-s,u)\tilde N_0(ds,du,dz)\Big|^{2\kappa}\Big] 
 \ar\leq\ar C \mathbf{E}\Big[ \Big|\int_0^t \int_{\mathbb{U}} \int_0^{Z(s-)} |R(t-s,u)|^2 N_0(ds,du,dz)\Big|^{\kappa}\Big].
 \eeqnn
 For $\kappa=1$, by the Cauchy-Schwarz inequality,
\beqnn
\lefteqn{ \mathbf{E}\Big[ \Big|\int_0^t \int_{\mathbb{U}} \int_0^{Z(s-)} R(t-s,u)\tilde N_0(ds,du,dz)\Big|^{2}\Big]}\ar\ar\cr
 \ar\leq\ar  C  \int_0^t\mathbf{E}[Z(s)]ds  \int_{\mathbb{U}}  |R(t-s,u)|^2 \nu_0(du)\cr
%\leq C \int_{\mathbb{U}\times\Psi}  \Big| \sup_{t\geq 0}R(t,u)\Big|^2 \nu_0(du,d\psi)
\ar\leq\ar C \int_{\mathbb{U}}   \sup_{r\geq 0}\phi(r,u) \nu_0(du)\int_0^\infty \phi(s,u)ds\cr
\ar\leq \ar C \int_{\mathbb{U}}   \sup_{r\geq 0}|\phi(r,u)|^2 \nu_0(du) +C \int_{\mathbb{U}}\Big|\int_0^\infty \phi(s,u)ds\Big|^2 \nu_0(du)<\infty.
\eeqnn
 %From (\ref{eqn4.13}) and Assumption~\ref{C1}(1),
 % \beqnn
 % \int_{\mathbb{U}\times\Psi}   \int_0^\infty |R_0(s,u)|^2 ds\nu_0(dk,d\mathbf{y})
 % \ar\leq\ar C \int_{\mathbb{U}\times\Psi}   k \int_0^\infty R_0(s,u) ds\nu_0(dk,d\mathbf{y})\cr
 % \ar\leq\ar C \int_{\mathbb{U}\times\Psi}   k\sum_{i=1}^j y_i \nu_0(dk,d\mathbf{y})<C.
 % \eeqnn
 Here the third inequality follows from  Lemma~\ref{Thm201} and (\ref{eqn4.06})-(\ref{eqn4.07}). 
 Taking these back into (\ref{eqnA.05.2}), we can get  $\sup_{t\geq 0}\mathbf{E}[|Z(t)|^2]<\infty$. 
 For $\kappa=\alpha$, 
  \beqlb\label{eqnA.07.00}
 \lefteqn{\mathbf{E}\Big[ \Big|\int_0^t \int_{\mathbb{U}} \int_0^{Z(s-)} R(t-s,u)\tilde N_0(ds,du,dz)\Big|^{2\alpha}\Big] }\ar\ar\cr
 \ar\leq\ar C \mathbf{E}\Big[ \Big|\int_0^t Z(s)ds \int_{\mathbb{U}} |R(t-s,u)|^2 \nu_0(du)\Big|^{\alpha}\Big]\cr
 \ar\ar + C \mathbf{E}\Big[ \Big|\int_0^t \int_{\mathbb{U}} \int_0^{Z(s-)} |R(t-s,u)|^2 \tilde{N}_0(ds,du,dz)\Big|^{\alpha}\Big].
 \eeqlb
 Applying Jensen's inequality to th first term on the right side of above inequality, we have 
 \beqlb\label{eqnA.07.01}
   \mathbf{E}\Big[ \Big|\int_0^t Z(s)ds \int_{\mathbb{U}} |R(t-s,u)|^2 \nu_0(du)\Big|^{\alpha}\Big]\ar\leq\ar  \int_{\mathbb{U}} \mathbf{E}\Big[ \Big|\int_0^t Z(s)|R(t-s,u)|^2 ds\Big|^{\alpha}\Big]\nu_0(du).
 \eeqlb
 From H\"older's inequality and the Cauchy-Schwarz inequality,
 \beqnn
 \mathbf{E}\Big[ \Big|\int_0^t Z(s)|R(t-s,u)|^2 ds\Big|^{\alpha}\Big]\ar\leq\ar \int_0^t\mathbf{E}[ |Z(s)|^\alpha] R(t-s,u) ds\cdot \Big|\int_0^t|R(r,u)|^{\frac{2\alpha-1}{\alpha-1}} dr\Big|^{\alpha-1}\cr
  \ar\leq\ar  \sup_{r\geq 0}|R(r,u)|^\alpha \Big|\int_0^t R(s,u) ds\Big|^\alpha \cr
 \ar\leq\ar \sup_{r\geq 0}|R(r,u)|^{2\alpha}  + \Big|\int_0^t R(s,u) ds\Big|^{2\alpha} .
 \eeqnn
 Taking this back into (\ref{eqnA.07.01}), from Condition~\ref{C1},
 \beqnn
\sup_{t\geq 0}  \mathbf{E}\Big[ \Big|\int_0^t Z(s)ds \int_{\mathbb{U}} |R(t-s,u)|^2 \nu_0(du)\Big|^{\alpha}\Big]<\infty.
 \eeqnn
 For the second term on the right of (\ref{eqnA.07.00}), by the Burkholder-Davis-Gundy inequality and the Cauchy-Schwarz inequality,
 \beqnn
 \lefteqn{ \mathbf{E}\Big[ \Big|\int_0^t \int_{\mathbb{U}} \int_0^{Z(s-)} |R(t-s,u)|^2 \tilde{N}_0(ds,du,dz)\Big|^{\alpha}\Big]}\ar\ar\cr
 \ar\leq\ar C  \mathbf{E}\Big[ \Big|\int_0^t \int_{\mathbb{U}} \int_0^{Z(s-)} |R(t-s,u)|^4  N_0(ds,du,dz)\Big|^{\alpha/2}\Big]\cr
 \ar\leq\ar  C\mathbf{E}\Big[  \int_0^t \int_{\mathbb{U}} \int_0^{Z(s-)} |R(t-s,u)|^{2\alpha} N_0(ds,du,dz)\Big]\cr
 \ar\leq\ar  \int_{\mathbb{U}}\nu_0(du)   \int_0^\infty |R(s,u)|^{2\kappa} ds \cr
 \ar\leq\ar \int_{\mathbb{U}} \nu_0(du) \sup_{r\geq 0} |R(r,u)|^{2\kappa-1}  \int_0^\infty R(s,u)ds\cr
 \ar\leq\ar \int_{\mathbb{U}}  \sup_{r\geq 0} |R(r,u)|^{2\kappa} \nu_0(du) +  \int_{\mathbb{U}} \Big|  \int_0^\infty R(s,u)ds  \Big|^{2\alpha}\nu_0(du)  .
 \eeqnn
 The boundedness for the last term follows  directly from (\ref{eqn4.06})-(\ref{eqn4.07}) and Condition~\ref{C1}.
 We have finished the proof.
 \qed
 
 \begin{corollary}\label{ThmA05}
 	There exists a constant $C>0$ such that for any $T\geq 0$,
 	\beqlb\label{eqnA.04.1}
 	\sup_{t\geq 0}\mathbf{E}\Big[ |\varepsilon_{T,H,2}(t)|^2\Big]\leq C\delta_T
 	\quad
 	\mbox{and}
 	\quad
 	\sup_{t\geq 0}\mathbf{E}\Big[ |\varepsilon_{T,H,2}(t)|^{2\alpha}\Big] \leq C|\delta_T|^\alpha.
 	\eeqlb
 	Moreover, the inequality (\ref{eqnA.04}) holds with $\gamma=\alpha$ for any $h\geq \delta_T/2$.
 \end{corollary}
 \proof  It is easy to see that the second result follows directly from the first one, i.e. by the Cauchy-Schwarz inequality, for any $h\geq \delta_T/2$,
 \beqnn
 \mathbf{E}\Big[ |\triangle_h\varepsilon_{T,H,2}(t)|^\alpha\times |\triangle_h\varepsilon_{T,H,2}(t+h)|^\alpha \Big]
 \ar\leq\ar C\mathbf{E}\Big[ |\varepsilon_{T,H,2}(t)|^{2\alpha}\Big] + C\mathbf{E}\Big[ |\varepsilon_{T,H,2}(t-h)|^{2\alpha} \Big]\cr
 \ar\ar\cr
 \ar\ar +C \mathbf{E}\Big[ |\varepsilon_{T,H,2}(t+h)|^{2\alpha}\Big]\leq C|\delta_T|^\alpha \leq Ch^\alpha.
 \eeqnn
 Now we start to prove the first result.
 %Let
 % \beqnn
 %  J(\xi)\ar=\ar \int_0^\xi \int_{\mathbb{U}\times\Psi} \int_0^{Z(Ts-)}
 %  \mathbf{1}_{s\geq {t-\delta_T}}\int_{T(t-s)}^\infty R_0(r,u)dr \tilde{N}_0(dTs,du,d\psi,d\psi,d\psidu,d\psi,d\psi,d\psi),
 % \eeqnn
 %  which is a  martingale.
 From the Burkholder-Davis-Gundy inequality, Lemma~\ref{Thm201} and (\ref{eqn4.07}),
 \beqnn
 \mathbf{E}\Big[ |\varepsilon_{T,H,2}(t)|^2\Big]
 \ar\leq\ar  \frac{1}{T}\mathbf{E}\Big[ \int_{t-\delta_T}^t  \int_{\mathbb{U}} \int_0^{Z(Ts-)}
 \Big|\int_{T(t-s)}^\infty R(r,u)dr\Big|^2 N_0(dTs,du,dz) \Big]\cr
 \ar\leq\ar
 C\int_{t-\delta_T}^t\mathbf{E}[Z(Ts)]ds  \int_{\mathbb{U}}
 \Big|\int_0^\infty R(r,u)dr\Big|^2  \nu_0(du)\leq C\delta_T.
 \eeqnn
 Similarly, applying the Burkholder-Davis-Gundy inequality and the Cauchy-Schwarz inequality, we also have
 \beqlb
 \mathbf{E}[ |\varepsilon_{T,H,2}(t)|^{2\alpha}]\ar\leq\ar
 \frac{C}{T^\alpha} \mathbf{E}\Big[ \Big| \int_{t-\delta_T}^t  \int_{\mathbb{U}}  \int_0^{Z(Ts-)}
 \Big|\int_0^\infty R(r,u)dr\Big|^2 N_0(dTs,du,dz)\Big|^\alpha \Big]\cr
 \ar\leq\ar
 \frac{C}{T^\alpha}\mathbf{E}\Big[ \Big| \int_{t-\delta_T}^t \int_{\mathbb{U}}  \int_0^{Z(Ts-)}
 \Big|\int_0^\infty R(r,u)dr\Big|^2 \tilde{N}_0(dTs,du,dz)\Big|^\alpha \Big]\cr
 \ar\ar +C\mathbf{E}\Big[ \Big| \int_{t-\delta_T}^t Z(Ts)ds
 \int_{\mathbb{U}}  \Big|\int_0^\infty R(r,u)dr\Big|^2 \nu_0(du)\Big|^\alpha \Big].\label{eqnA.05.1}
 \eeqlb
 For the second term on the right side of the last inequality, from (\ref{eqn4.07}) and H\"older's inequality,
 \beqnn
 \lefteqn{\mathbf{E}\Big[ \Big| \int_{t-\delta_T}^t Z(Ts)ds
 	\int_{\mathbb{U}}  \Big|\int_0^\infty R(r,u)dr\Big|^2 \nu_0(du)\Big|^\alpha \Big]}\ar\ar\cr
 \ar\leq\ar C\mathbf{E}\Big[ \Big| \int_{t-\delta_T}^t Z(Ts)ds\Big|^\alpha \Big]\leq C |\delta_T|^{\alpha-1} \int_{t-\delta_T}^t \mathbf{E}[|Z(Ts)|^\alpha]ds \leq C |\delta_T|^{\alpha}.
 \eeqnn
 For the first term, applying the Burkholder-Davis-Gundy inequality again, we have
 \beqlb\label{eqnA.06.1}
 \lefteqn{ \frac{1}{T^\alpha}\mathbf{E}\Big[ \Big| \int_{t-\delta_T}^t \int_{\mathbb{U}}  \int_0^{Z(Ts-)}
 	\Big|\int_0^\infty R(r,u)dr\Big|^2 \tilde{N}_0(dTs,du,dz)\Big|^\alpha \Big]}\ar\ar\cr
 \ar\leq\ar  \frac{C}{T^\alpha}\mathbf{E}\Big[ \Big| \int_{t-\delta_T}^t \int_{\mathbb{U}}  \int_0^{Z(Ts-)}
 \Big|\int_0^\infty R(r,u)dr\Big|^4 N_0(dTs,du,dz)\Big|^{\alpha/2} \Big]\cr
 \ar\leq\ar  \frac{C}{T^\alpha}\mathbf{E}\Big[   \int_{t-\delta_T}^t \int_{\mathbb{U}}  \int_0^{Z(Ts-)}
 \Big|\int_0^\infty R(r,u)dr\Big|^{2\alpha} N_0(dTs,du,dz)  \Big]\cr
 \ar\leq\ar  \frac{C}{T^{\alpha-1}}   \int_{t-\delta_T}^t
 \mathbf{E}[Z(Ts)] ds
 \int_{\mathbb{U}}  \Big|\int_0^\infty R(r,u)dr\Big|^{2\alpha} \nu_0(du)\leq CT^{1-\beta-\alpha}.
 \eeqlb
 Here the second inequality follows from the fact that $\alpha/2\leq 1$.
 Taking these two estimates above back into (\ref{eqnA.05.1}), we will get the desired result directly.
 \qed

 Now we start to prove that (\ref{eqnA.04}) also holds when $h< \delta_T/2$. In this case, we can see that $t-h-\delta_T<t-\delta_T<t+h-\delta_T<t-h< t<t+h $, which suggest us to split the interval of integration  $\varepsilon_{T,H,2}(t+h)$ into the following three disjoint parts:
 \beqnn
 \varepsilon_{T,H,2}(t+h)\ar=\ar  \frac{1}{\sqrt{T}} \int_{t}^{t+h} \int_{\mathbb{U}}   \int_0^{Z(Ts-)}
 \int_{T(t+h-s)}^\infty R(r,u)dr\tilde{N}_0(dTs,du,dz)\cr
 \ar\ar +  \frac{1}{\sqrt{T}} \int_{t-h}^{t} \int_{\mathbb{U}}  \int_0^{Z(Ts-)}
 \int_{T(t+h-s)}^\infty R(r,u)dr\tilde{N}_0(dTs,du,dz)\cr
 \ar\ar +  \frac{1}{\sqrt{T}} \int_{t+h-\delta_T}^{t-h} \int_{\mathbb{U}}   \int_0^{Z(Ts-)}
 \int_{T(t+h-s)}^\infty R(r,u)dr\tilde{N}_0(dTs,du,dz).
 \eeqnn
 The decompositions for $\varepsilon_{T,H,2}(t)$ and $\varepsilon_{T,H,2}(t-h)$ can be given similarly. Thus
 \beqnn
 \triangle_h\varepsilon_{T,H,2}(t+h)
 \ar=\ar \sum_{i=1}^4 I_{T,i}(t,h)\quad \mbox{and}\quad \triangle_h\varepsilon_{T,H,2}(t)=\sum_{j=5}^8 I_{T,j}(t,h),
 \eeqnn
 where
 \beqnn
 I_{T,1}(t,h)\ar=\ar  \frac{1}{\sqrt{T}} \int_{t}^{t+h} \int_{\mathbb{U}}  \int_0^{Z(Ts-)}
 \int_{T(t+h-s)}^\infty R(r,u)dr\tilde{N}_0(dTs,du,dz),\cr
 I_{T,2}(t,h)\ar=\ar -  \frac{1}{\sqrt{T}} \int_{t-h}^{t} \int_{\mathbb{U}}  \int_0^{Z(Ts-)}
 \int_{T(t-s)}^{T(t+h-s)} R(r,u)dr\tilde{N}_0(dTs,du,dz),\cr
 I_{T,3}(t,h)\ar=\ar -  \frac{1}{\sqrt{T}} \int_{t+h-\delta_T}^{t-h} \int_{\mathbb{U}}  \int_0^{Z(Ts-)}
 \int_{T(t-s)}^{T(t+h-s)} R(r,u)dr\tilde{N}_0(dTs,du,dz),\cr
 I_{T,4}(t,h)\ar=\ar - \frac{1}{\sqrt{T}} \int_{t-\delta_T}^{t+h-\delta_T} \int_{\mathbb{U}}  \int_0^{Z(Ts-)}
 \int_{T(t-s)}^\infty R(r,u)dr\tilde{N}_0(dTs,du,dz)
 \eeqnn
 and
 \beqnn
 I_{T,5}(t,h)\ar=\ar  \frac{1}{\sqrt{T}} \int_{t-h}^t \int_{\mathbb{U}}  \int_0^{Z(Ts-)}
 \int_{T(t-s)}^\infty R(r,u)dr\tilde{N}_0(dTs,du,dz),\cr
 I_{T,6}(t,h)\ar=\ar  -  \frac{1}{\sqrt{T}} \int_{t+h-\delta_T}^{t-h} \int_{\mathbb{U}}  \int_0^{Z(Ts-)}
 \int_{T(t-h-s)}^{T(t-s)} R(r,u)dr\tilde{N}_0(dTs,du,dz),\cr
 I_{T,7}(t,h)\ar=\ar  - \frac{1}{\sqrt{T}} \int_{t-\delta_T}^{t+h-\delta_T} \int_{\mathbb{U}}  \int_0^{Z(Ts-)}
 \int_{T(t-h-s)}^{T(t-s)} R(r,u)dr\tilde{N}_0(dTs,du,dz),\cr
 I_{T,8}(t,h)\ar=\ar  -  \frac{1}{\sqrt{T}} \int_{t-h-\delta_T}^{t-\delta_T} \int_{\mathbb{U}}  \int_0^{Z(Ts-)}
 \int_{T(t-h-s)}^\infty R(r,u)dr\tilde{N}_0(dTs,du,dz).\cr
 \eeqnn
 From the Cauchy-Schwarz inequality,
 \beqnn
 \mathbf{E}\Big[ |\triangle_h\varepsilon_{T,H,2}(t)|^\alpha\times |\triangle_h\varepsilon_{T,H,2}(t+h)|^\alpha \Big]
 \ar\leq\ar C\sum_{i=1}^4\sum_{j=5}^8 \mathbf{E}\big[|I_{T,i}(T,h)|^\alpha \cdot |I_{T,j}(T,h)|^\alpha\big].
 \eeqnn
 Thus it suffices to prove that every expectation in the summation can be bounded by $Ch^{\gamma}$ for some constants $C>0$ and $\gamma>1$ independent of $T$, $t$ and $h$.
 
 \begin{corollary}\label{ThmA06}
 	There exists a constant $C>0$  such that  for any $t\in[0,1]$ and $h>0$,
 	\beqnn
 	\sum_{i\in\{1,2,4\}}\sum_{j\in\{5,7,8\}} \mathbf{E}\big[|I_{T,i}(t,h)|^\alpha \cdot |I_{T,j}(t,h)|^\alpha\big]\leq Ch^{\alpha\wedge \frac{3}{2}}.
 	\eeqnn
 \end{corollary}
 \proof Here we just consider the case $i=1$ and $j=5$. Other cases can be proved similarly.
 Like the argument in the proof of Corollary~\ref{ThmA05}, there exists a constant $C>0$ such that
 \beqlb\label{eqnA.05}
 \mathbf{E}[|I_{T,1}(t,h)|^{2\alpha}]+ \mathbf{E}[|I_{T,5}(t,h)|^{2\alpha}]\leq C\frac{(Th)^{\alpha}+Th}{T^\alpha}.
 \eeqlb
 When $Th\geq 1$, by H\"older's inequality,
 \beqnn
 \mathbf{E}\big[|I_{T,1}(t,h)|^\alpha \cdot |I_{T,5}(t,h)|^\alpha\big]\ar\leq\ar  \Big(\mathbf{E}\big[|I_{T,1}(t,h)|^{2\alpha}\big] \cdot  \mathbf{E}\big[|I_{T,5}(t,h)|^{2\alpha}\big]\Big)^{1/2} \leq Ch^\alpha.
 \eeqnn
 Now we consider the case $Th< 1$.
 For any $\xi\geq 0$, define
 \beqnn
 J_1(\xi)\ar:=\ar \int_{t}^\xi \int_{\mathbb{U}}  \int_0^{Z(Ts-)}\mathbf{1}_{\{s\in(t,t+h]\}}
 \int_{T(t+h-s)}^\infty R(r,u)dr\tilde{N}_0(dTs,du,dz),\cr
 J_2(\xi)\ar:=\ar \int_{t-h}^\xi \int_{\mathbb{U}}  \int_0^{Z(Ts-)} \mathbf{1}_{\{s\in(t-h,t]\}}
 \int_{T(t-s)}^\infty R(r,u)dr\tilde{N}_0(dTs,du,dz),
 \eeqnn
 which are two $(\mathscr{F}_{T\cdot})$-martingales for any $t$ and $h$ fixed.
 Following the argument of conditional expectation, we have
 \beqlb\label{eqnA.06}
 \mathbf{E}\big[|I_{T,1}(t,h)|^\alpha \cdot |I_{T,5}(t,h)|^\alpha\big]
 \ar=\ar\frac{1}{T^\alpha}\mathbf{E}\big[|J_1(t+h)|^\alpha|J_2(t)|^\alpha\big]\cr
 \ar=\ar\frac{1}{T^\alpha} \mathbf{E}\big[|J_2(t)|^\alpha \cdot \mathbf{E}_{\mathscr{F}_{Tt}}[|J_1(t+h)|^\alpha]\big].
 \eeqlb
 Like the deduction in (\ref{eqnA.06.1}),
 from the Burkholder-Davis-Gundy inequality and (\ref{eqn4.07}), there exists a constant $C>0$ such that
 \beqnn
 \mathbf{E}_{\mathscr{F}_{Tt}}[|J_1(t+h)|^\alpha]
 \ar\leq\ar CT\int_{t}^{t+h} \mathbf{E}_{\mathscr{F}_{Tt}}[Z(Ts)]ds
 \eeqnn
 and
 \beqnn
 \mathbf{E}[|J_1(t+h)|^\alpha|J_2(t)|^\alpha]\ar\leq \ar CT\int_{t}^{t+h} \mathbf{E}\big[|J_2(t)|^\alpha \cdot \mathbf{E}_{\mathscr{F}_{Tt}}[Z(Ts)]\big]ds\cr
 \ar\leq\ar CT\int_{t}^{t+h}
 \mathbf{E}[|J_2(t)|^\alpha Z(Ts-)]ds.
 \eeqnn
 By H\"older's inequality, Lemma~\ref{ThmA04} and (\ref{eqnA.05}),
 \beqnn
 \mathbf{E}[|J_1(t+h)|^\alpha|J_2(t)|^\alpha]\ar\leq\ar CT\int_{t}^{t+h}
 \sqrt{\mathbf{E}[|J_2(t)|^{2\alpha}]\cdot\mathbf{E}[ |Z(Ts)|^2]}ds\cr
 \ar\leq\ar  CTh
 \sqrt{\mathbf{E}[|J_2(t)|^{2\alpha}]}\leq CT^{3/2}h^{3/2}.
 \eeqnn
 Taking this back into (\ref{eqnA.06}), we have
 \beqnn
 \mathbf{E}\big[|I_{T,1}(t,h)|^\alpha \cdot |I_{T,5}(t,h)|^\alpha\big]\leq CT^{3/2-\alpha}h^{3/2}\leq \left\{
 \begin{array}{ll}
 	Ch^{3/2}, & \mbox{if }\alpha\geq 3/2;\vspace{7pt}\\
 	C h^\alpha, & \mbox{if }1<\alpha<3/2.
 \end{array}
 \right.
 \eeqnn
 Here we have finished the proof.
 \qed

 \begin{corollary}\label{ThmA07}
 	There exist constants $C>0$ and $\gamma\in(1,\alpha(1+\beta)/2)$  such that  for any $t\in[0,1]$ and $h>0$,
 	\beqnn
 	\sum_{i\in\{1,2,4\}}\mathbf{E}\big[|I_{T,i}(t,h)|^\alpha \cdot |I_{T,6}(t,h)|^\alpha\big]+\sum_{j\in\{5,7,8\}} \mathbf{E}\big[|I_{T,3}(t,h)|^\alpha \cdot |I_{T,j}(t,h)|^\alpha\big]\leq Ch^{\gamma}.
 	\eeqnn
 \end{corollary}
 \proof Here we just prove this result with $i=1$ and $j=6$. Other cases can be proved in the same way.
 Like the argument in the proof of Corollary~\ref{ThmA05}, there exists a constant $C>0$ such that
 \beqlb\label{eqnA.07}
 \mathbf{E}\big[|I_{T,1}(t,h)|^{2\alpha}\big] \leq C\frac{(Th)^\alpha+ Th}{T^\alpha}\quad \mbox{and}\quad \mathbf{E}\big[|I_{T,6}(t,h)|^{2\alpha}\big] \leq C|\delta_T|^\alpha.
 \eeqlb
 When $Th\geq 1$, by H\"older's inequality,
 \beqnn
 \mathbf{E}\big[|I_{T,1}(t,h)|^{\alpha}\cdot |I_{T,6}(t,h)|^{\alpha}\big]\leq C |\delta_T|^{\alpha/2} h^{\alpha/2}\leq CT^{-\beta\alpha/2}h^{\alpha/2}\leq Ch^{\alpha(1+\beta)/2}.
 \eeqnn
 Since $\beta>2/\alpha-1$, then (\ref{eqnA.04}) holds with $\gamma=\alpha(1+\beta)/2>1$ since $\alpha\beta>1$.
 When $Th<1$,  (\ref{eqnA.07}) induces directly that
 \beqnn
 \mathbf{E}\big[|I_{T,1}(t,h)|^{2\alpha}\big]\leq CT^{1-\alpha}h.
 \eeqnn
 Moreover, from the Burkholder-Davis-Gundy inequality  and (\ref{eqn4.06}),
 \beqlb
 \mathbf{E}[|I_{T,6}(t,h)|^{2\alpha}]
 \ar\leq\ar  \frac{C}{T^\alpha}\mathbf{E}\Big[ \Big|\int_{t+h-\delta_T}^{t-h} \int_{\mathbb{U}}  \int_0^{Z(Ts-)}
 \Big|\int_{T(t-h-s)}^{T(t-s)} R(r,u)dr\Big|^2N_0(dTs,du,dz)\Big|^{\alpha} \Big]\cr
 \ar\leq\ar CT^\alpha h^{2\alpha} \mathbf{E}\Big[ \Big|\int_{t+h-\delta_T}^{t-h} \int_{\mathbb{U}}  \int_0^{Z(Ts-)}\sup_{r\geq 0}|\phi(r,u)|^2N_0(dTs,du,dz)\Big|^{\alpha} \Big].\label{eqnA.10.1}
 \eeqlb
 Like the deduction in (\ref{eqnA.06.1}), we also have
 \beqlb\label{eqnA.08}
 \mathbf{E}[|I_{T,6}(t,h)|^{2\alpha}] \ar\leq\ar  C T^\alpha h^{2\alpha}\big((T\delta_T)^\alpha+T\delta_T\big)\leq C (Th)^{2\alpha} |\delta_T|^\alpha.
 \eeqlb
 From these estimates and H\"older's inequality,
 \beqnn
 \mathbf{E}[|I_{T,1}(t,h)|^{\alpha}|I_{T,6}(t,h)|^{\alpha}]\leq C T^{1/2+\alpha(1-\beta)/2}  h^{1/2+\alpha}
 \eeqnn
 Since $\gamma\in(1,\alpha(1+\beta)/2)$ and $h\leq 1/T$, thus
 \beqnn
 \mathbf{E}[|I_{T,1}(t,h)|^{\alpha}|I_{T,6}(t,h)|^{\alpha}]\leq C T^{1+\gamma-\alpha(1+\beta)/2}  h^{1+\gamma}\leq C h^{1+\gamma}.
 \eeqnn
 Here we have finished the proof.
 \qed

 \begin{corollary}\label{ThmA08}
 	There exist a constant $C>0$  such that for any $h<\delta_T/2$ and $T>0$,
 	\beqnn
 	\mathbf{E}[|I_{T,3}(t,h)|^{\alpha}|I_{T,6}(t,h)|^{\alpha}]\leq Ch^{\alpha\beta}.
 	\eeqnn
 \end{corollary}
 \proof From (\ref{eqnA.07}) and (\ref{eqnA.08}), we have
 \beqnn
 \mathbf{E}[|I_{T,3}(t,h)|^{2\alpha}]+\mathbf{E}[ |I_{T,6}(t,h)|^{2\alpha}] \leq
 \left\{  \begin{array}{ll}
 	C|\delta_T|^\alpha, & \mbox{if }Th\geq 1;\vspace{5pt}\\
 	C (Th)^{2\alpha} |\delta_T|^\alpha, & \mbox{if }Th< 1.
 \end{array}
 \right.
 \eeqnn
 By H\"older's inequality, when $Th\geq 1$,
 \beqnn
 \mathbf{E}[|I_{T,3}(t,h)|^\alpha|I_{T,6}(t,h)|^\alpha]\ar\leq\ar \Big( \mathbf{E}[|I_{T,3}(t,h)|^{2\alpha}]\mathbf{E}[ |I_{T,6}(t,h)|^{2\alpha}] \Big)^{1/2}\leq   C |\delta_T|^\alpha \leq C h^{\alpha\beta}
 \eeqnn
 and when $Th<1$,
 \beqnn
 \mathbf{E}[|I_{T,3}(t,h)|^\alpha|I_{T,6}(t,h)|^\alpha]\ar\leq\ar C T^{2\alpha-\beta \alpha} h^{2\alpha}\leq C (Th)^{2\alpha-\beta \alpha} h^{\alpha\beta}\leq Ch^{\alpha\beta}.
 \eeqnn
 Here we have finished the proof.
 \qed

 \section{Proof for Lemma~\ref{Thm405}}\label{AppendixB}
 \setcounter{equation}{0}

In this subsection we just show the detailed proof for the weak convergence of the sequence $\{\sqrt{T}\varepsilon^\psi_{T,H}(\cdot)\}_{T\geq 0}$ to $0$ in the space $\mathbb{D}([0,\infty),\mathbb{R})$ under Condition~\ref{C1} and \ref{C2}.
 The weak convergence of $\{\sqrt{T}\varepsilon^\psi_{T,I}(\cdot)\}_{T\geq 0}$ can be proved similarly. 
 Redefine $\delta_T:=T^{-\beta}$ with $\beta\in(\frac{1}{\alpha}, 1-\frac{1}{2\theta_1})$. We split the error process $\sqrt{T}\varepsilon^\psi_{T,H}(\cdot)$ into the following two parts:
 \beqlb
 \varepsilon^\psi_{T,H,1}(t)\ar:=\ar  \frac{1}{\sqrt{T}}\int_0^{t-\delta_T} \int_{\mathbb{U}}  \psi^{\mathrm{c}}(T(t-s),u) N_H(dTs,du),\quad \label{eqnA.12}\\
 \varepsilon^\psi_{T,H,2}(t)\ar:=\ar  \frac{1}{\sqrt{T}}\int_{t-\delta_T}^{t} \int_{\mathbb{U}} \psi^{\mathrm{c}}(T(t-s),u) N_H(dTs,du).\label{eqnA.13}
 \eeqlb
 Fro the first term, we have 
 \beqlb
  |\varepsilon^\psi_{T,H,1}(t)|\ar\leq\ar \frac{1}{\sqrt{T}}\int_0^{t-\delta_T} \int_{\mathbb{U}}  \sup_{s\leq t-\delta_T }|\psi^{\mathrm{c}}(T(t-s),u)| N_H(dTs,du)\cr
  \ar\leq\ar  \frac{1}{\sqrt{T}}\int_0^{t-\delta_T} \int_{\mathbb{U}}  \sup_{s\geq T^{1-\beta}}|\psi^{\mathrm{c}}(s,u) | N_H(dTs,du).
 \eeqlb
 From Lemma~\ref{Thm201} and Condition~\ref{C2},
 \beqlb
 \mathbf{E}\Big[ \sup_{t\in[0,1]}  |\varepsilon^\psi_{T,H,1}(t)| \Big] \ar\leq\ar  \sqrt{T}\int_0^1 \mathbf{E}[ Z(Ts)]ds \int_{\mathbb{U}}  \sup_{s\geq T^{1-\beta}}|\psi^{\mathrm{c}}(s,u) | \nu_0(du)\leq  T^{\frac{1}{2} -\theta_1(1-\beta)} ,
 \eeqlb
 which vanishes as $T\to\infty$.  
 Now we start to consider $\varepsilon^\psi_{T,H,2}(\cdot)$. For any $t\geq 0$, 
 \beqlb
  |\varepsilon^\psi_{T,H,2}(t)|\ar\leq \ar  \frac{1}{\sqrt{T}}\int_{t-\delta_T}^{t} \int_{\mathbb{U}} |\psi^{\mathrm{c}}(T(t-s),u) |N_H(dTs,du)\cr
  \ar\leq\ar  \frac{1}{\sqrt{T}}\int_{t-\delta_T}^{t} \int_{\mathbb{U}}\sup_{r\geq 0} |\psi^{\mathrm{c}}(r,u) |N_H(dTs,du).
 \eeqlb 
Thus the proof will be end if the following statement holds: for any $\epsilon>0$, we have as $T\to\infty$,
\beqlb\label{eqnA.19}
 \mathbf{P}\Big\{\sup_{t\in[0,1]}  \frac{1}{\sqrt{T}}\int_{t-\delta_T}^{t} \int_{\mathbb{U}}\sup_{r\geq 0} |\psi^{\mathrm{c}}(r,u) |N_H(dTs,du)>\epsilon \Big\} \to 0.
\eeqlb
Indeed, this probability can be bounded by
\beqnn
 \lefteqn{ \mathbf{P}\Big\{ \sup_{i=0,\cdots [T^\beta]-1}\frac{1}{\sqrt{T}} \int_{iT^{-\beta}}^{(i+2)T^{-\beta}} \int_{\mathbb{U}}\sup_{r\geq 0} |\psi^{\mathrm{c}}(r,u) |N_H(dTs,du)>\epsilon \Big\}}\ar\ar\cr
\ar\leq\ar  \sum_{i=0}^{ [T^\beta]-1}\mathbf{P}\Big\{ \frac{1}{\sqrt{T}} \int_{iT^{1-\beta}}^{(i+2)T^{1-\beta}} \int_{\mathbb{U}}\sup_{r\geq 0} |\psi^{\mathrm{c}}(r,u) |N_H(ds,du)>\epsilon \Big\}\cr
\ar\leq\ar  \sum_{i=0}^{ [T^\beta]-1}\frac{1}{T^\alpha \epsilon^{2\alpha}} \mathbf{E}\Big[ \Big| \int_{iT^{1-\beta}}^{(i+2)T^{1-\beta}} \int_{\mathbb{U}}\sup_{r\geq 0} |\psi^{\mathrm{c}}(r,u) |N_H(ds,du)\Big|^{2\alpha} \Big].
\eeqnn
Here the last inequality follows from Chebyshev's inequality. 
From the Cauchy-Schwarz inequality, 
\beqlb\label{eqnB.07}
\lefteqn{\mathbf{E}\Big[ \Big| \int_{iT^{1-\beta}}^{(i+2)T^{1-\beta}} \int_{\mathbb{U}}\sup_{r\geq 0} |\psi^{\mathrm{c}}(r,u) |N_H(ds,du)\Big|^{2\alpha} \Big]}\ar\ar\cr
\ar\leq\ar C\mathbf{E}\Big[ \Big| \int_{iT^{1-\beta}}^{(i+2)T^{1-\beta}} Z(s)ds\int_{\mathbb{U}}\sup_{r\geq 0} |\psi^{\mathrm{c}}(r,u) |\nu_0(du)\Big|^{2\alpha} \Big]\cr
\ar\ar + C\mathbf{E}\Big[ \Big| \int_{iT^{1-\beta}}^{(i+2)T^{1-\beta}} \int_{\mathbb{U}}\sup_{r\geq 0} |\psi^{\mathrm{c}}(r,u) |\tilde{N}_H(ds,du)\Big|^{2\alpha} \Big].
\eeqlb
From Condition~\ref{C2}, H\"older's ineqaulity and Corollary~\ref{ThmA04}, we can see that  
\beqlb\label{eqnB.08}
\lefteqn{\mathbf{E}\Big[ \Big| \int_{iT^{1-\beta}}^{(i+2)T^{1-\beta}} Z(s)ds\int_{\mathbb{U}}\sup_{r\geq 0} |\psi^{\mathrm{c}}(r,u) |\nu_0(du)\Big|^{2\alpha} \Big]}\ar\ar\cr
\ar\leq\ar 
C\mathbf{E}\Big[ \Big| \int_{iT^{1-\beta}}^{(i+2)T^{1-\beta}} Z(s)ds\Big|^{2\alpha} \Big]
\leq C T^{(2\alpha-1)(1-\beta)} \int_{iT^{1-\beta}}^{(i+2)T^{1-\beta}}\mathbf{E}[ |Z(s)|^{2\alpha} ] ds\leq CT^{2\alpha(1-\beta)}.
\eeqlb
From the  Burkholder-Davis-Gundy inequality and  the Cauchy-Schwarz inequality to the second term on the right side of  (\ref{eqnB.07}),  
\beqlb\label{eqnB.09}
\lefteqn{\mathbf{E}\Big[ \Big| \int_{iT^{1-\beta}}^{(i+2)T^{1-\beta}} \int_{\mathbb{U}}\sup_{r\geq 0} |\psi^{\mathrm{c}}(r,u) |\tilde{N}_H(ds,du)\Big|^{2\alpha} \Big]}\ar\ar\cr
\ar \leq\ar  C\mathbf{E}\Big[ \Big| \int_{iT^{1-\beta}}^{(i+2)T^{1-\beta}} \int_{\mathbb{U}}\sup_{r\geq 0} |\psi^{\mathrm{c}}(r,u) |^2N_H(ds,du)\Big|^{\alpha} \Big]\cr
\ar\leq\ar  C\mathbf{E}\Big[ \Big| \int_{iT^{1-\beta}}^{(i+2)T^{1-\beta}} Z(s)ds\int_{\mathbb{U}}\sup_{r\geq 0} |\psi^{\mathrm{c}}(r,u) |^2\nu_0(du)\Big|^{\alpha} \Big] \cr
\ar\ar +C\mathbf{E}\Big[ \Big| \int_{iT^{1-\beta}}^{(i+2)T^{1-\beta}} \int_{\mathbb{U}}\sup_{r\geq 0} |\psi^{\mathrm{c}}(r,u) |^2\tilde{N}_H(ds,du)\Big|^{\alpha} \Big].
\eeqlb
Like the deduction in (\ref{eqnB.08}), we also have 
\beqlb\label{eqnB.10}
\mathbf{E}\Big[ \Big| \int_{iT^{1-\beta}}^{(i+2)T^{1-\beta}} Z(s)ds\int_{\mathbb{U}}\sup_{r\geq 0} |\psi^{\mathrm{c}}(r,u) |^2\nu_0(du)\Big|^{\alpha} \Big]
\ar\leq\ar  C T^{\alpha(1-\beta)}.
\eeqlb
Applying the  Burkholder-Davis-Gundy inequality again to the last term in (\ref{eqnB.09}), we have 
\beqnn
 C\mathbf{E}\Big[ \Big| \int_{iT^{1-\beta}}^{(i+2)T^{1-\beta}} \int_{\mathbb{U}}\sup_{r\geq 0} |\psi^{\mathrm{c}}(r,u) |^2\tilde{N}_H(ds,du)\Big|^{\alpha} \Big] 
\ar\leq\ar C\mathbf{E}\Big[ \Big| \int_{iT^{1-\beta}}^{(i+2)T^{1-\beta}} \int_{\mathbb{U}}\sup_{r\geq 0} |\psi^{\mathrm{c}}(r,u) |^4N_H(ds,du)\Big|^{\alpha/2} \Big]\cr
\ar\leq\ar  C\mathbf{E}\Big[   \int_{iT^{1-\beta}}^{(i+2)T^{1-\beta}} \int_{\mathbb{U}}\sup_{r\geq 0} |\psi^{\mathrm{c}}(r,u) |^{2\alpha}N_H(ds,du) \Big]\cr
\ar=\ar C \int_{iT^{1-\beta}}^{(i+2)T^{1-\beta}} \mathbf{E}[Z(s)]ds\leq CT^{1-\beta}.
\eeqnn
Putting all estimates above together, we have 
\beqnn
\mathbf{P}\Big\{\sup_{t\in[0,1]}  |\varepsilon^\psi_{T,H,2}(t)|>\epsilon \Big\} \leq  \frac{ C}{ \epsilon^{2\alpha}}T^{\alpha   -(2\alpha-1)\beta}.
\eeqnn
which vanishes as $T\to\infty$ since $\beta>\frac{\alpha}{2\alpha-1}$. Here we have gotten (\ref{eqnA.19}) and the proof for Lemma~\ref{Thm405} have been finished.

 %
 %
 % Moreover, we have
 % \beqnn
 % \varepsilon_{T,2,2}(t)\ar\leq\ar \frac{C}{\sqrt{T}} \int_{T(t-\delta_T)}^{Tt} (Z(s)+\mathbf{E}[Z(s)])ds\leq \frac{C}{\sqrt{T}} \int_{T(t-\delta_T)}^{Tt} Z(s)ds+ C\sqrt{T}\delta_T.
 % \eeqnn
 % For any $\epsilon>0$
 % \beqnn
 % \mathbf{P}\Big\{\sup_{t\in[0,1]} \frac{1}{\sqrt{T}} \int_{T(t-\delta_T)}^{Tt} Z(s)ds>\epsilon \Big\} \ar\leq\ar  \mathbf{P}\Big\{ \sup_{i=0,\cdots [T^\beta]-1}\frac{1}{\sqrt{T}} \int_{iT\delta_T}^{(i+2)T\delta_T} Z(s)ds>\epsilon \Big\}\cr
 % \ar\leq\ar  \sum_{i=0}^{ [T^\beta]-1}\mathbf{P}\Big\{ \frac{1}{\sqrt{T}} \int_{iT\delta_T}^{(i+2)T\delta_T} Z(s)ds>\epsilon \Big\}
 % \eeqnn
 % Here
 % \beqnn
 % \mathbf{P}\Big\{ \frac{1}{\sqrt{T}} \int_{iT\delta_T}^{(i+2)T\delta_T} Z(s)ds>\epsilon \Big\}\ar\leq\ar \frac{1}{T^\alpha \epsilon^{2\alpha}} \mathbf{E}\Big[ \Big|  \int_{iT\delta_T}^{(i+2)T\delta_T} Z(s)ds\Big|^{2\alpha} \Big]\cr
 % \ar\leq\ar \frac{C}{T^\alpha \epsilon^{2\alpha}}  (T\delta_T)^{2\alpha-1} \int_{iT\delta_T}^{(i+2)T\delta_T} \mathbf{E}[|Z(s)|^ {2\alpha}] ds\cr
 % \ar\leq\ar  \frac{C}{T^\alpha \epsilon^{2\alpha}}  (T\delta_T)^{2\alpha}\leq \frac{C}{  \epsilon^{2\alpha}}  T^{\alpha-2\beta\alpha}
 % \eeqnn
 % and
 % \beqnn
 % \mathbf{P}\Big\{ \frac{1}{\sqrt{T}} \int_{iT\delta_T}^{(i+2)T\delta_T} Z(s)ds>\epsilon \Big\}\ar\leq\ar \frac{C}{  \epsilon^{2\alpha}}  T^{\alpha+\beta-2\beta\alpha}
 % \eeqnn
 % Here we need $\beta>\alpha/(2\alpha-1)$ and $\theta>1+\frac{1}{2\alpha-2}$.
 % \qed
